# Supplementary material for: Data-driven prediction and control of extreme events in a chaotic flow
Source: arXiv:2204.11682 source file (2022-04-25)
Supplement: Supplementary file 1 [file supp_mat.tex]

% \unappendix
\setcounter{page}{1}
\setcounter{figure}{0}
\setcounter{section}{18}% Equivalent to "letter O"
\section{supplementary material}
\subsection{Block Diagrams}

In this section, we show mathematically detailed block diagrams versions of the block diagrams reported in the main text.  

\begin{figure}[H]
\centering
\includegraphics[width=.9\textwidth]{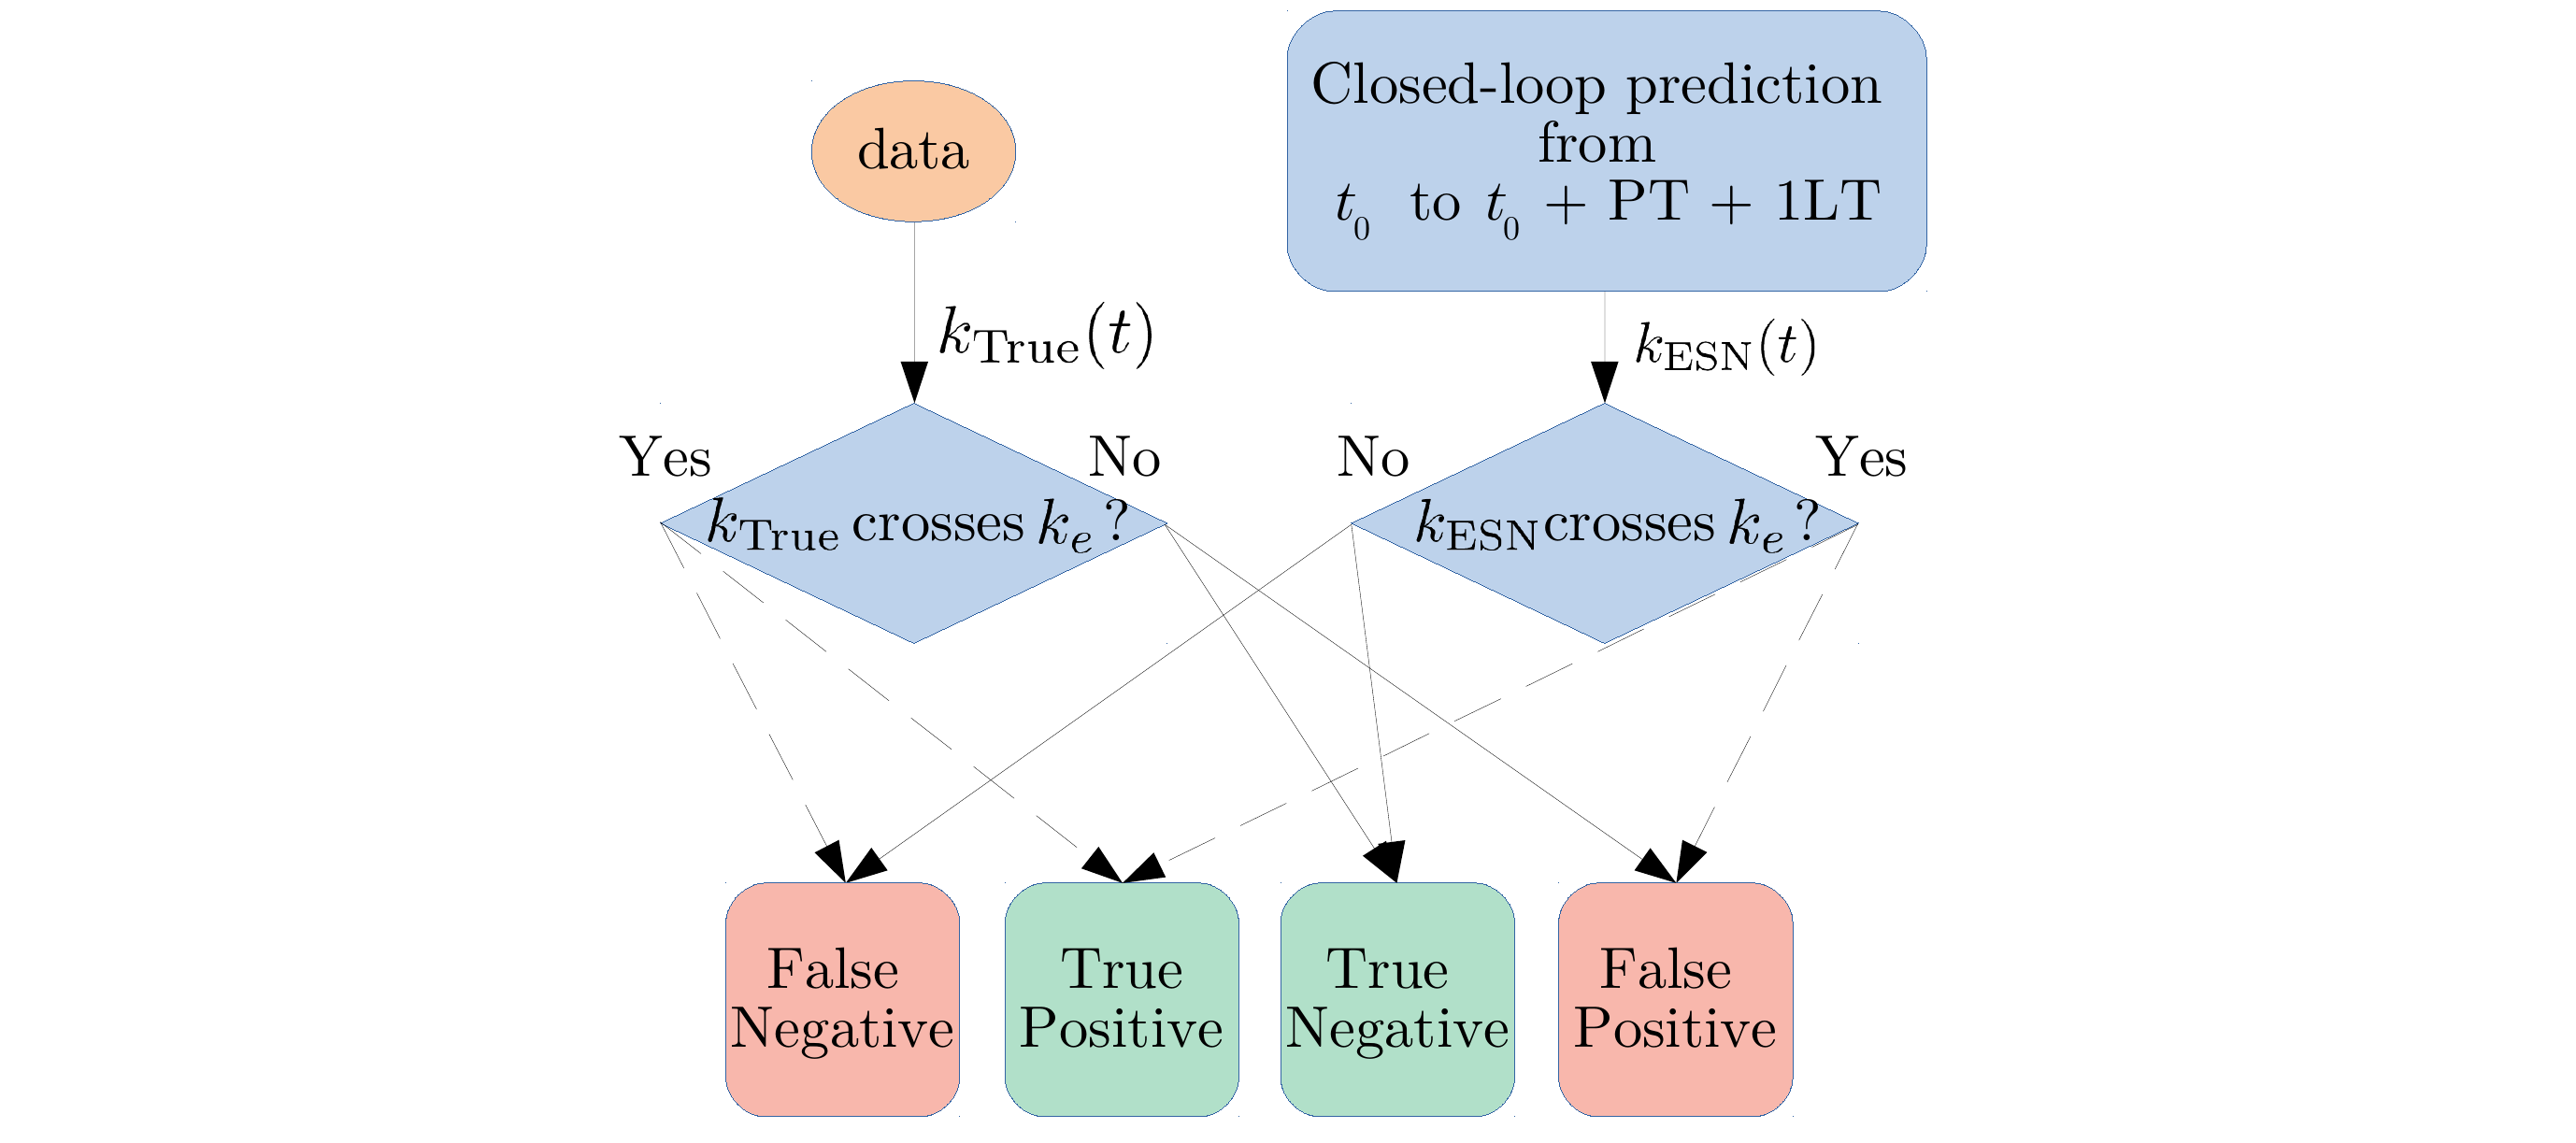}
\caption{Schematic representation of the prediction of extreme events with echo state networks. For a starting point, $t_0$, we evaluate whether the predicted kinetic energy, $k_{\mathrm{ESN}}$, and the true kinetic energy, $k_{\mathrm{True}}$, cross the extreme event threshold, $k_e$, in the interval $[t_0+\mathrm{PT},t_0+\mathrm{PT} + 1\mathrm{LT}]$, where PT is the prediction time.}
\label{fig:pr_scheme_supp}
\end{figure}

\begin{figure}[H]
\centering
\includegraphics[width=.9\textwidth]{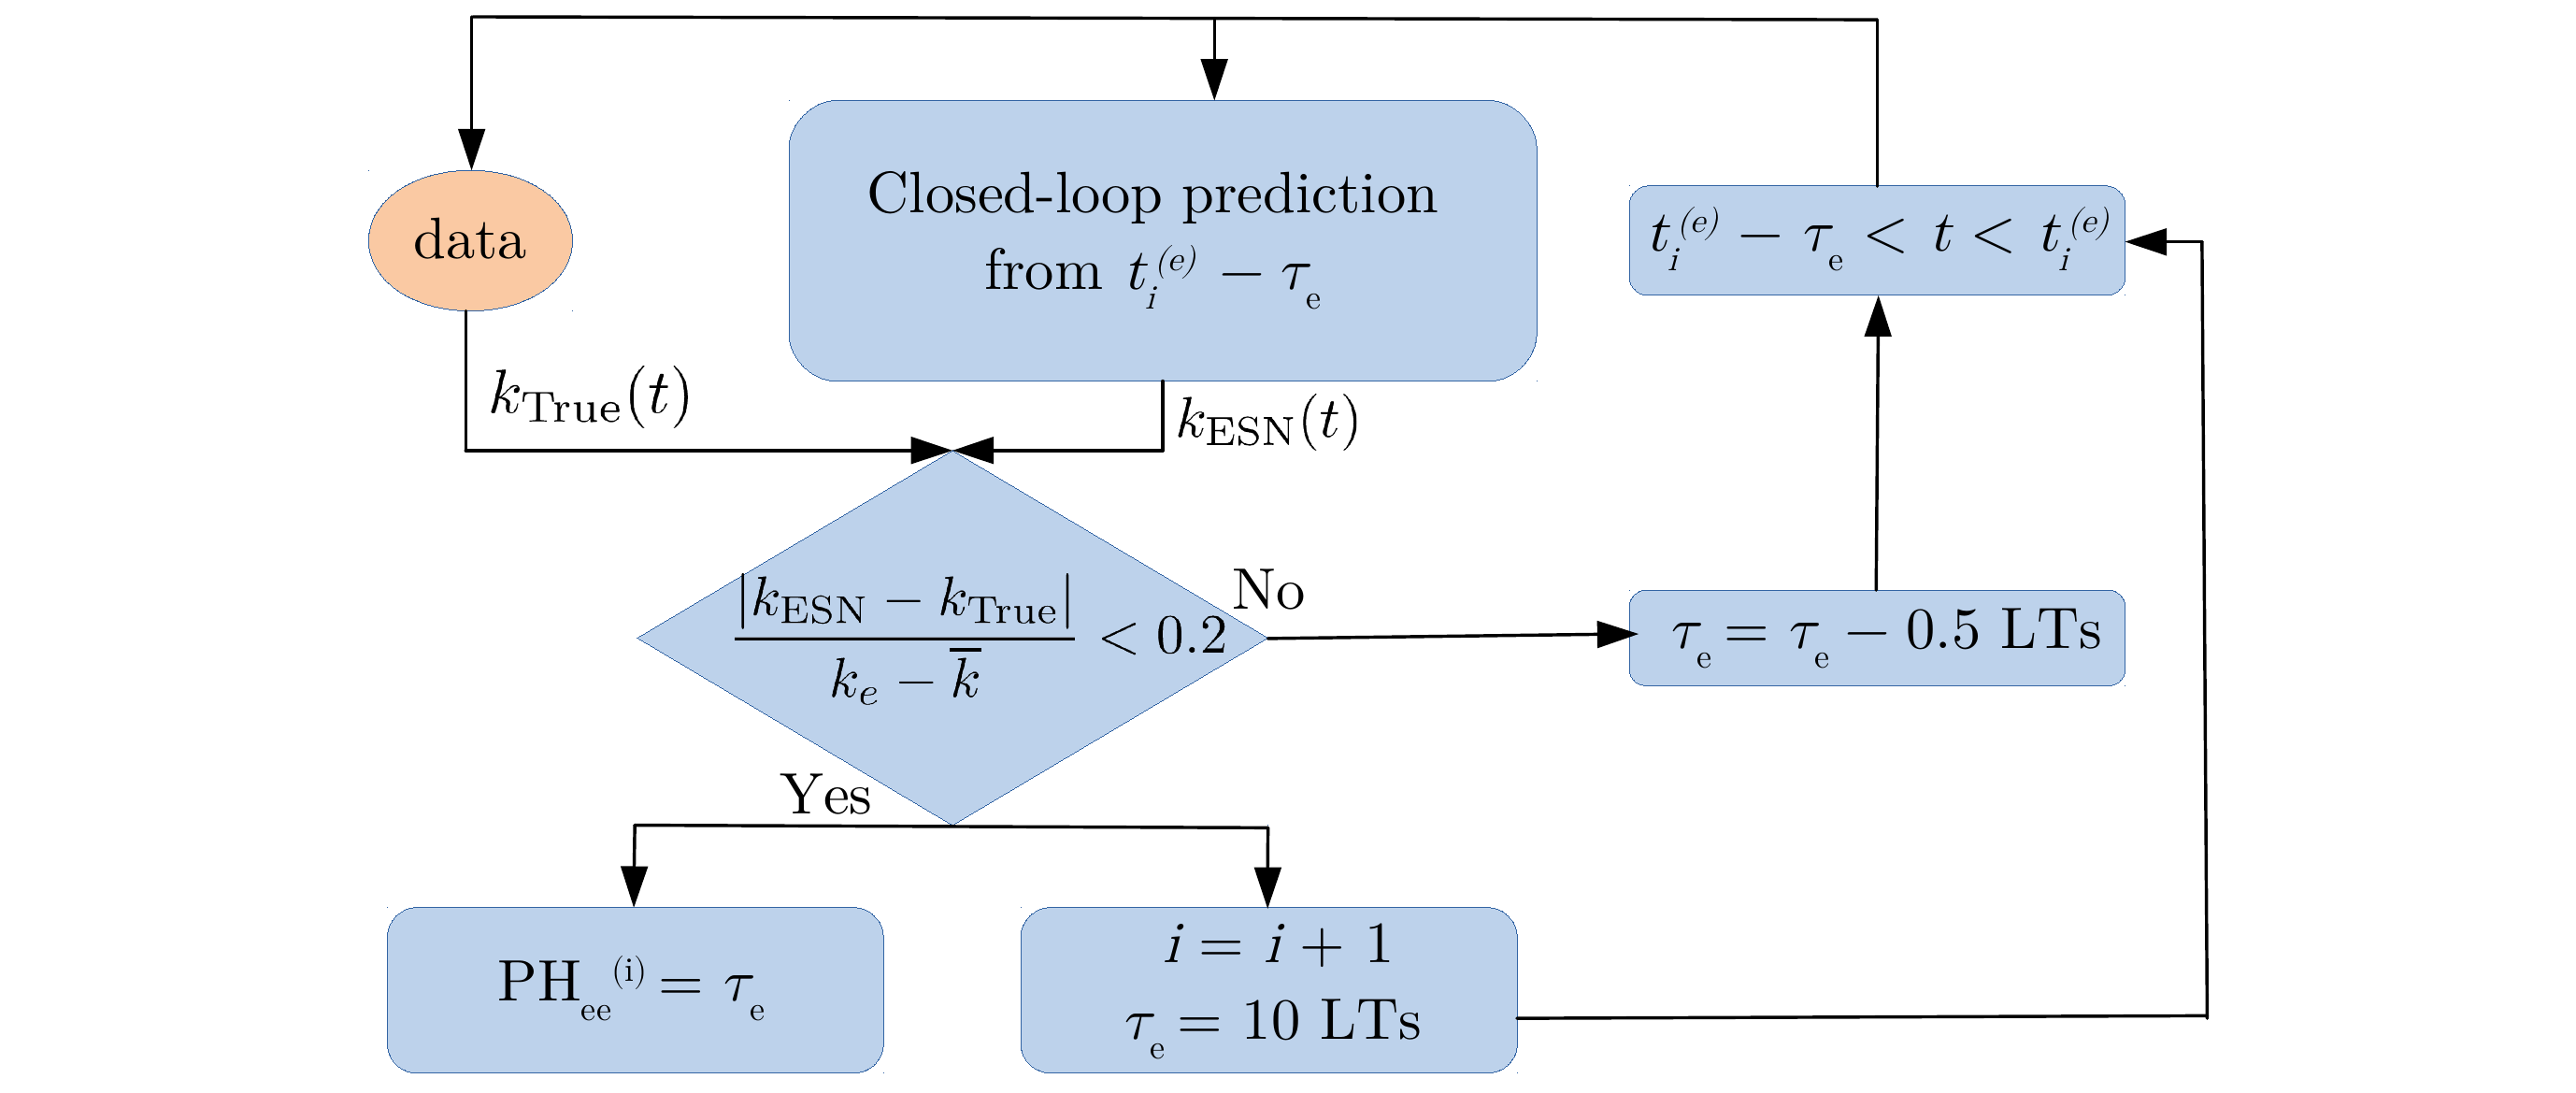}
\caption{Schematic representation of the computation of the prediction horizon for extreme events, $\mathrm{PH}_{\mathrm{ee}}$. For the $i-$th event, we evaluate if the prediction horizon \eqref{eq:PH} of the closed-loop prediction starting from $\tau_e$ before the event is larger than $\tau_e$, which is initialized  to 10LTs. If the prediction horizon is larger, $\mathrm{PH}_{\mathrm{ee}}=\tau_e$ and we analyze the next event, if not, we decrease $\tau_e$ by 0.5LTs and evaluate the prediction horizon starting from the new $\tau_e$ before the event.}
\label{fig:phee_scheme_supp}
\end{figure}

\begin{figure}[H]
\centering
\includegraphics[width=.9\textwidth]{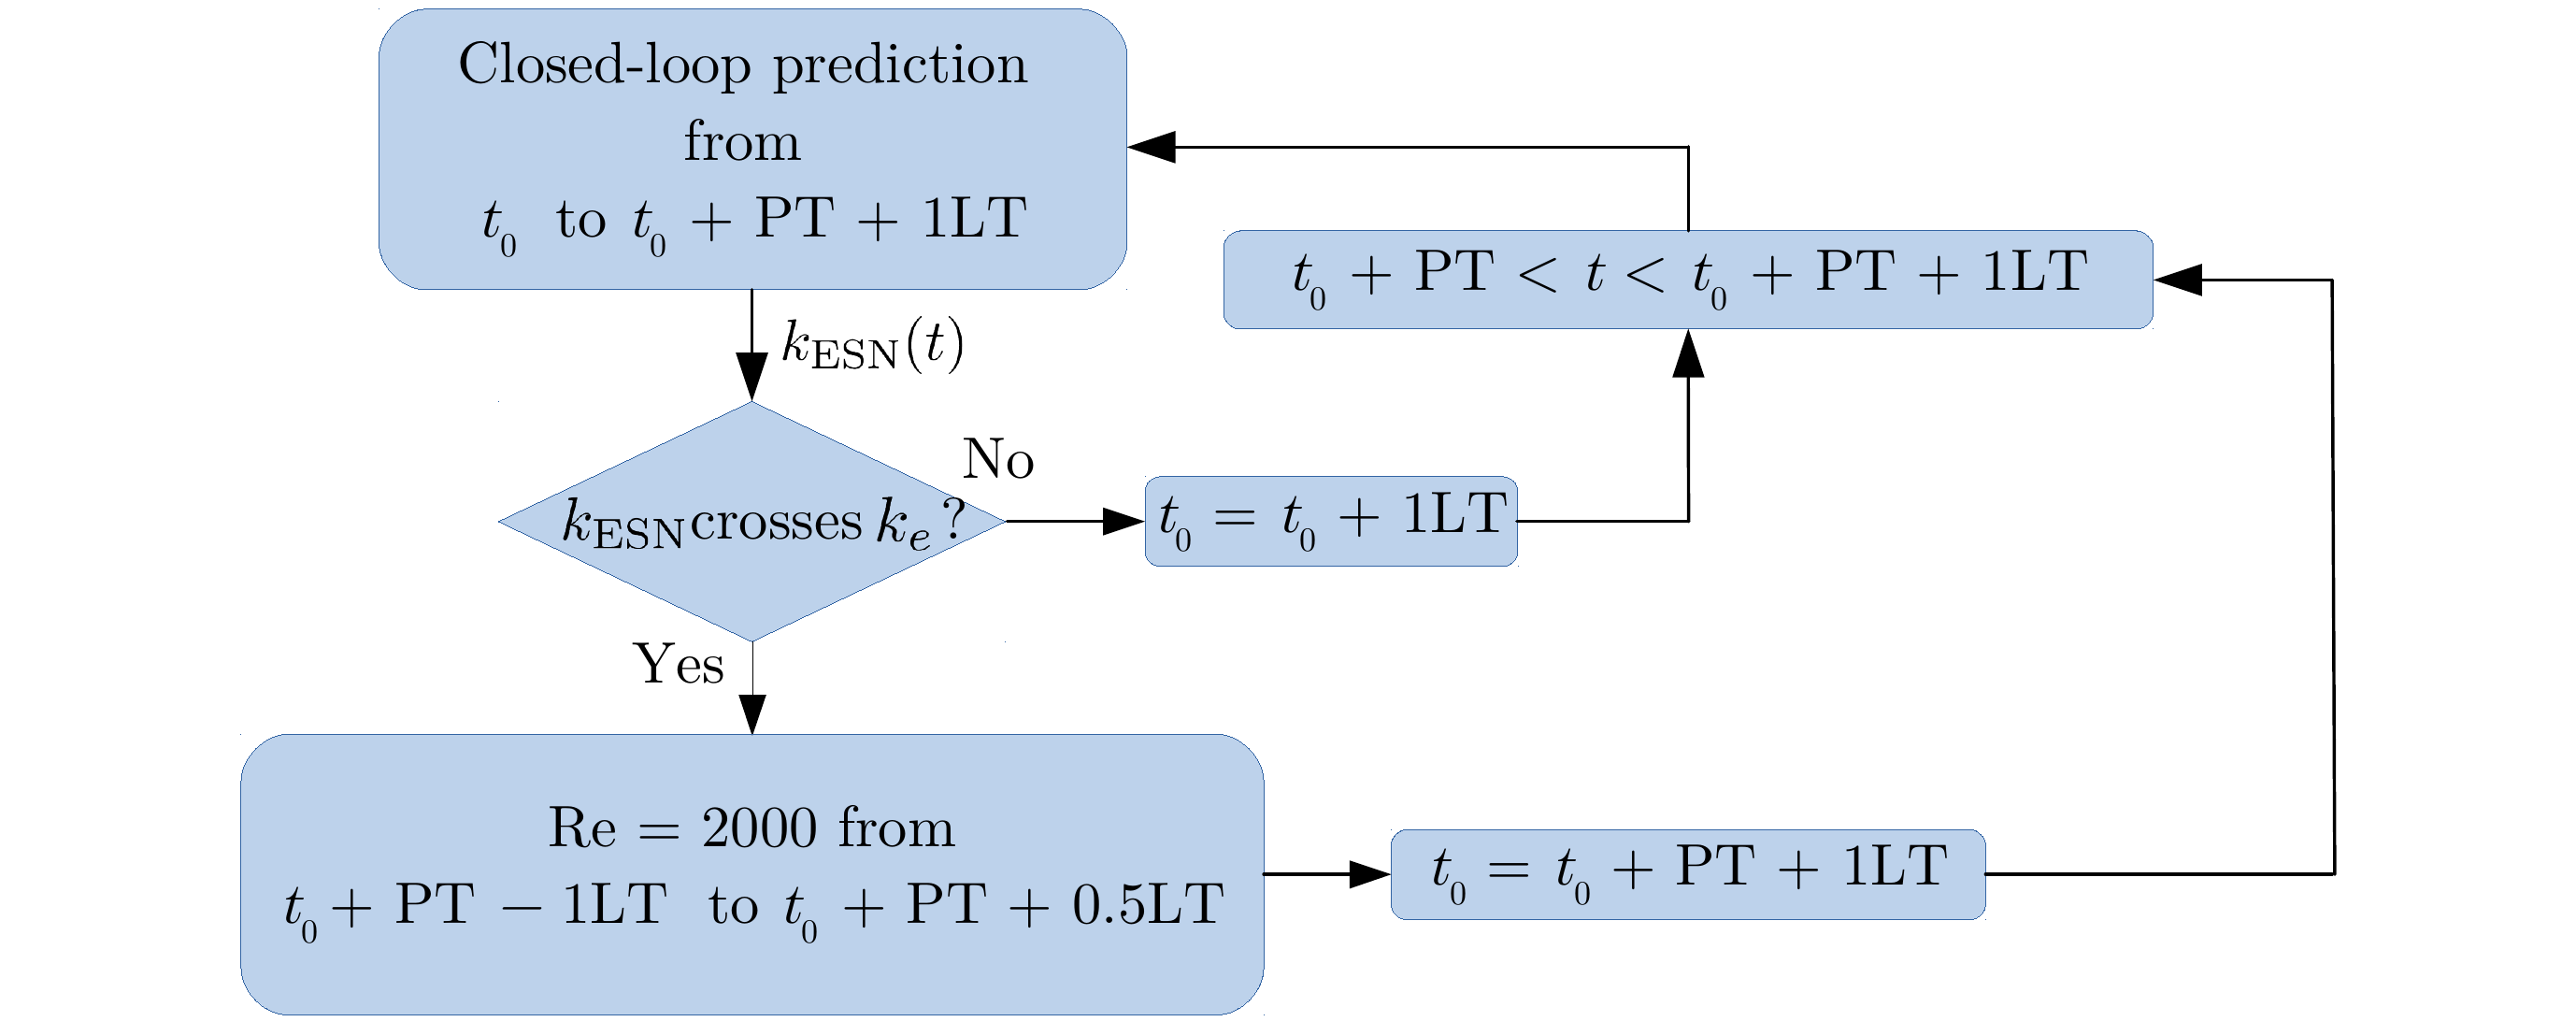}
\caption{Schematic representation of the control strategy. If the ESN closed-loop starting at $t_0$ predicts an event in the interval $t_0+[\mathrm{PT},\mathrm{PT}+1\mathrm{LTs}]$, we increase the Reynolds number to 2000 from $t_0+\mathrm{PT}-1\mathrm{LTs}$ to $t_0+\mathrm{PT}+0.5\mathrm{LTs}$. The next closed-loop prediction then starts after the control strategy ends at the updated $t_0=t_0+\mathrm{PT}+0.5\mathrm{LTs}$.}
\label{fig:control_scheme_supp}
\end{figure}

\subsection{Reduced-order model}
\label{sec:reduced}

The nine modes of the MFE model \cite{moehlis2004low} described in section \ref{sec:MFE} are:

\begin{enumerate}
\item The basic profile:
\begin{equation}
\mathbf{\hat{v}_1} = \left( \begin{array}{c} \sqrt{2}\sin(\pi y/2)\\0\\0
\end{array} \right)
\end{equation}
\item The streak:
\begin{equation}
\mathbf{\hat{v}_2} = \left( \begin{array}{c}
\frac{4}{\sqrt{3}} \cos^2(\pi y/2) \cos(\gamma z)\\
0\\
0
\end{array} \right)
\end{equation}
\item The downstream vortex:
\begin{equation}
\mathbf{\hat{v}_3} = \frac{2}{\sqrt{4\gamma^2 + \pi^2}} \left( \begin{array}{c}
0\\
2\gamma \cos(\pi y/2) \cos(\gamma z)\\
\pi \sin(\pi y/2) \sin(\gamma z)
\end{array} \right)
\end{equation}
\item The spanwise flows:
\begin{equation}
\mathbf{\hat{v}_4} = \left( \begin{array}{c}
0\\
0\\
\frac{4}{\sqrt{3}} \cos(\alpha x) \cos^2(\pi y/2)
\end{array} \right)
\end{equation}
\begin{equation}
\mathbf{\hat{v}_5} = \left( \begin{array}{c}
0\\
0\\
2 \sin(\alpha x) \sin(\pi y/2)
\end{array} \right)
\end{equation}
\item The normal vortex modes:
\begin{equation}
\mathbf{\hat{v}_6} = \frac{4\sqrt{2}}{\sqrt{3(\alpha^2+\gamma^2)}}
\left( \begin{array}{c}
-\gamma\cos(\alpha x) \cos^2(\pi y/2) \sin(\gamma z) \\
0\\
\alpha \sin(\alpha x) \cos^2(\pi y/2) \cos(\gamma z)
\end{array} \right)
\end{equation}
\begin{equation}
\mathbf{\hat{v}_7} = \frac{2\sqrt{2}}{\sqrt{\alpha^2+\gamma^2}}
\left( \begin{array}{c}
\gamma\sin(\alpha x) \sin(\pi y/2) \sin(\gamma z) \\
0\\
\alpha \cos(\alpha x) \sin(\pi y/2) \cos(\gamma z)
\end{array} \right)
\end{equation}
\item A three-dimensional mode:
\begin{equation}
\mathbf{\hat{v}_8} = N_8
\left( \begin{array}{c}
\pi \alpha \sin(\alpha x) \sin(\pi y/2) \sin(\gamma z)\\
2(\alpha^2+\gamma^2) \cos(\alpha x) \cos(\pi y/2) \sin(\gamma z)\\
-\pi \gamma \cos(\alpha x) \sin(\pi y/2) \cos(\gamma z)
\end{array} \right)
\end{equation}
with 
\begin{equation}
N_8 = \frac{2\sqrt{2}}{\sqrt{(\alpha^2 + \gamma^2)(4\alpha^2 + 4\gamma^2 + \pi^2)}}
\end{equation}
\item The modification of the basic profile mode:
\begin{equation}
\mathbf{\hat{v}_9} = \left( \begin{array}{c}
\sqrt{2}\sin(3\pi y/2)\\
0\\
0
\end{array} \right)
\end{equation}

\end{enumerate}

The governing equations for the modes are:

\begin{equation}
\frac{da_1}{dt} = \frac{\beta^2}{Re} - \frac{\beta^2}{Re}a_1 - \sqrt{\frac{3}{2}} \frac{\beta \gamma}{\kappa_{\alpha \beta \gamma}}a_6 a_8 + \sqrt{\frac{3}{2}} \frac{\beta \gamma}{\kappa_{\beta \gamma}}a_2 a_3
\end{equation}
\begin{align}
\frac{da_2}{dt} = -\left( \frac{4\beta^2}{3} + \gamma^2 \right) \frac{a_2}{Re} + \frac{5\sqrt{2}}{3\sqrt{3}} \frac{\gamma^2}{\kappa_{\alpha \gamma}} a_4 a_6 - \frac{\gamma^2}{\sqrt{6} \kappa_{\alpha \gamma}} a_5 a_7 \nonumber \\
		-\frac{\alpha \beta \gamma}{\sqrt{6} \kappa_{\alpha \gamma} \kappa_{\alpha \beta \gamma}} a_5 a_8 - \sqrt{\frac{3}{2}} \frac{\beta \gamma}{\kappa_{\beta \gamma}} a_1 a_3 - \sqrt{\frac{3}{2}} \frac{\beta \gamma}{\kappa_{\beta \gamma}} a_3 a_9
\end{align}

\begin{align}
\frac{da_3}{dt} = - \frac{\beta^2 + \gamma^2}{Re} a_3 + \frac{2}{\sqrt{6}} \frac{\alpha \beta \gamma}{\kappa_{\alpha \gamma} \kappa_{\beta \gamma}}(a_4 a_7 + a_5 a_6) + \frac{\beta^2(3\alpha^2 + \gamma^2) - 3\gamma^2 (\alpha^2 + \gamma^2)}{\sqrt{6} \kappa_{\alpha\gamma} \kappa_{\beta \gamma} \kappa_{\alpha \beta \gamma}} a_4 a_8
\end{align}
\begin{align}
\frac{da_4}{dt} = & - \frac{3\alpha^2 + 4\beta^2}{3 Re} a_4 - \frac{\alpha}{\sqrt{6}} a_1 a_5 - \frac{10}{3\sqrt{6}} \frac{\alpha^2}{\kappa_{\alpha\gamma}} a_2 a_6 \nonumber \\
	&- \sqrt{\frac{3}{2}} \frac{\alpha \beta \gamma}{\kappa_{\alpha\gamma}\kappa_{\beta\gamma}} a_3 a_7 - \sqrt{\frac{3}{2}} \frac{\alpha^2 \beta^2}{\kappa_{\alpha\gamma}\kappa_{\beta\gamma}\kappa_{\alpha\beta\gamma}}a_3 a_8 - \frac{\alpha}{\sqrt{6}}a_5 a_9
\end{align}
\begin{align}
\frac{da_5}{dt} = - \frac{\alpha^2 + \beta^2}{Re}a_5 + \frac{\alpha}{\sqrt{6}} a_1 a_4 + \frac{\alpha^2}{\sqrt{6}} a_1 a_4 + \frac{\alpha^2}{\sqrt{6}\kappa_{\alpha\gamma}}a_2 a_7 \nonumber \\
	- \frac{\alpha \beta \gamma}{\sqrt{6} \kappa_{\alpha \gamma}\kappa_{\alpha\beta\gamma}}a_2 a_8 + \frac{\alpha}{\sqrt{6}} a_4 a_9 + \frac{2}{\sqrt{6}} \frac{\alpha \beta \gamma}{\kappa_{\alpha\gamma}\kappa_{\beta\gamma}} a_3 a_6
\end{align}
\begin{align}
\frac{da_6}{dt} =& - \frac{3\alpha^2 + 4\beta^2 + 3\gamma^2}{3Re}a_6 + \frac{\alpha}{\sqrt{6}} a_1 a_7 + \sqrt{\frac{3}{2}} \frac{\beta \gamma}{\kappa_{\alpha\beta\gamma}} a_1 a_8 \nonumber \\
	&+ \frac{10}{3\sqrt{6}} \frac{\alpha^2 - \gamma^2}{\kappa_{\alpha\gamma}} a_2 a_4 - 2\sqrt{\frac{2}{3}} \frac{\alpha\beta\gamma}{\kappa_{\alpha\gamma}\kappa_{\beta\gamma}}a_3 a_5 + \frac{\alpha}{\sqrt{6}}a_7a_9 + \sqrt{\frac{3}{2}} \frac{\beta \gamma}{\kappa_{\alpha\beta\gamma}}a_8a_9
\end{align}
\begin{align}
\frac{da_7}{dt} = -\frac{\alpha^2 + \beta^2 + \gamma^2}{Re} a_7 - \frac{\alpha}{\sqrt{6}} (a_1 a_6 + a_6 a_9) + \frac{1}{\sqrt{6}} \frac{\gamma^2 - \alpha^2}{\kappa_{\alpha\gamma}} a_2 a_5 + \frac{1}{\sqrt{6}} \frac{\alpha \beta \gamma}{\kappa_{\alpha\gamma}\kappa{\beta\gamma}}a_3a_4
\end{align}
\begin{align}
\frac{da_8}{dt} =  -\frac{\alpha^2 + \beta^2 + \gamma^2}{Re} a_8 + \frac{2}{\sqrt{6}} \frac{\alpha \beta \gamma}{\kappa_{\alpha\gamma}\kappa_{\alpha\beta\gamma}}a_2a_5 + \frac{\gamma^2(3\alpha^2-\beta^2+3\gamma^2)}{\sqrt{6}\kappa_{\alpha\gamma}\kappa_{\beta\gamma}\kappa_{\alpha\beta\gamma}}a_3a_4
\end{align}
\begin{align}
\frac{da_9}{dt} = -\frac{9\beta^2}{Re}a_9 + \sqrt{\frac{3}{2}} \frac{\beta\gamma}{\kappa_{\beta\gamma}}a_2a_3 - \sqrt{\frac{3}{2}} \frac{\beta\gamma}{\kappa_{\alpha\beta\gamma}} a_6a_8
\end{align}
where
\begin{gather}
\kappa_{\alpha\gamma} = \sqrt{\alpha^2+\gamma^2}, \quad
\kappa_{\beta\gamma} = \sqrt{\beta^2+\gamma^2}, \quad
\kappa_{\alpha\beta\gamma} = \sqrt{\alpha^2+\beta^2+\gamma^2} \nonumber \\
\nonumber \\
\alpha = \frac{2\pi}{L_x}, \quad
\beta = \frac{\pi}{2}, \quad
\gamma = \frac{2\pi}{L_z}.
\end{gather}
